# Supplementary material for: Thermodynamically Consistent Machine-Learned Internal State Variable Approach for Data-Driven Modeling of Path-Dependent Materials
Source: arXiv:2205.00578 source file (2022-05-01)
Supplement: Supplementary file 1 [file sec7-appendix.tex]

\section{xxx}\label{sec:appendix}
